# Supplementary material for: MPLP++: Fast, Parallel Dual Block-Coordinate Ascent for Dense Graphical Models
Source: arXiv:2004.08227 source file (2020-04-16)
Supplement: Supplementary file 1 [file eccv2018_supplementary.tex]

% last updated in April 2002 by Antje Endemann
% Based on CVPR 07 and LNCS, with modifications by DAF, AZ and elle, 2008 and AA, 2010, and CC, 2011; TT, 2014; AAS, 2016

\documentclass[runningheads]{llncs}
\usepackage{graphicx}
\usepackage{amsmath,amssymb} % define this before the line numbering.
\usepackage{ruler}
\usepackage{color}
\usepackage[width=122mm,left=12mm,paperwidth=146mm,height=193mm,top=12mm,paperheight=217mm]{geometry}

%	USE PACKAGE
%	USE PACKAGE

% use Times
\usepackage{times}
% For figures
\usepackage{graphicx} % more modern
\usepackage{subfigure} 

% For citations
%\usepackage{natbib}

% For algorithms
\usepackage{algorithm}
\usepackage{algorithmic}

% As of 2011, we use the hyperref package to produce hyperlinks in the
% resulting PDF.  If this breaks your system, please commend out the
% following usepackage line and replace \usepackage{icml2017} with
% \usepackage[nohyperref]{icml2017} above.
\usepackage{hyperref}

% Packages hyperref and algorithmic misbehave sometimes.  We can fix
% this with the following command.

\usepackage{times}
\usepackage{epsfig}
\usepackage{graphicx}
\usepackage{xcolor}
\usepackage{subfiles}
\usepackage{bm}
\usepackage{multirow}
\usepackage{array}

%\documentclass{article}

% use Times
\usepackage{times}
% For figures
\usepackage{graphicx} % more modern
\usepackage{subfigure} 

% For citations
\usepackage[numbers]{natbib}

%% For algorithms
%\usepackage{algorithm}
%\usepackage{algorithmic}
%
%% As of 2011, we use the hyperref package to produce hyperlinks in the
%% resulting PDF.  If this breaks your system, please commend out the
%% following usepackage line and replace \usepackage{icml2017} with
%% \usepackage[nohyperref]{icml2017} above.
%\usepackage{hyperref}

% Packages hyperref and algorithmic misbehave sometimes.  We can fix
% this with the following command.
%\newcommand{\theHalgorithm}{\arabic{algorithm}}
%\newcommand{\floor}[1]{\lfloor #1 \rfloor}

%\usepackage{times}
%\usepackage{epsfig}
%%\usepackage{stmaryrd}
%\usepackage{graphicx}
%%\usepackage{amsmath}
%%\usepackage{amssymb}
%\usepackage{amsthm}
%\usepackage{xcolor}
%%\usepackage{algorithm}
%%\usepackage{algorithmic}
%%\usepackage{mathtools,algorithm}
%%\usepackage[noend]{algpseudocode}
%\usepackage{subfiles}
%%\usepackage{algorithm2e}
%%\usepackage{tabularx}
%%\usepackage[noend]{algpseudocode}
%\usepackage{bm}
%\usepackage{multirow}
%\usepackage{array}

%
% Theorem environments
%
%\newtheorem{definition}{Definition}
%\newtheorem{theorem}{Theorem}
%\newtheorem{lemma}{Lemma}
%\newtheorem{proposition}{Proposition}
%\newtheorem{corollary}{Corollary}
%\newtheorem{example}{Example}
%\newcommand\dataF[1]{\texttt{\textbf{ #1}}}

%
% Math
%

%\newcommand\SX{\mathcal X}

\newcommand\TRWS{\texttt{TRW-S} }

\newcommand\HaSh{\texttt{MPLP}++ }

\begin{document}
% \renewcommand\thelinenumber{\color[rgb]{0.2,0.5,0.8}\normalfont\sffamily\scriptsize\arabic{linenumber}\color[rgb]{0,0,0}}
% \renewcommand\makeLineNumber {\hss\thelinenumber\ \hspace{6mm} \rlap{\hskip\textwidth\ \hspace{6.5mm}\thelinenumber}}
% \linenumbers
\pagestyle{headings}
\mainmatter
\def\ECCV18SubNumber{***}  % Insert your submission number here

\title{MPLP++: Fast Parallelizable Dual Block-Coordinate Ascent for \\ Dense Graphical Models - Supplementary} % Replace with your title

\titlerunning{ECCV-18 submission ID \ECCV18SubNumber}

\authorrunning{ECCV-18 submission ID \ECCV18SubNumber}

\author{Anonymous ECCV submission}
\institute{Paper ID \ECCV18SubNumber}

\maketitle

\begin{figure*}
\centering
%\begin{subfigure}[Protein Folding]{
%\includegraphics[width=0.18\linewidth]{./plots/protein_folding/protein_folding_dual_iters}
%}
%\end{subfigure}
\begin{subfigure}[Worms]
{\includegraphics[width=0.30\linewidth]{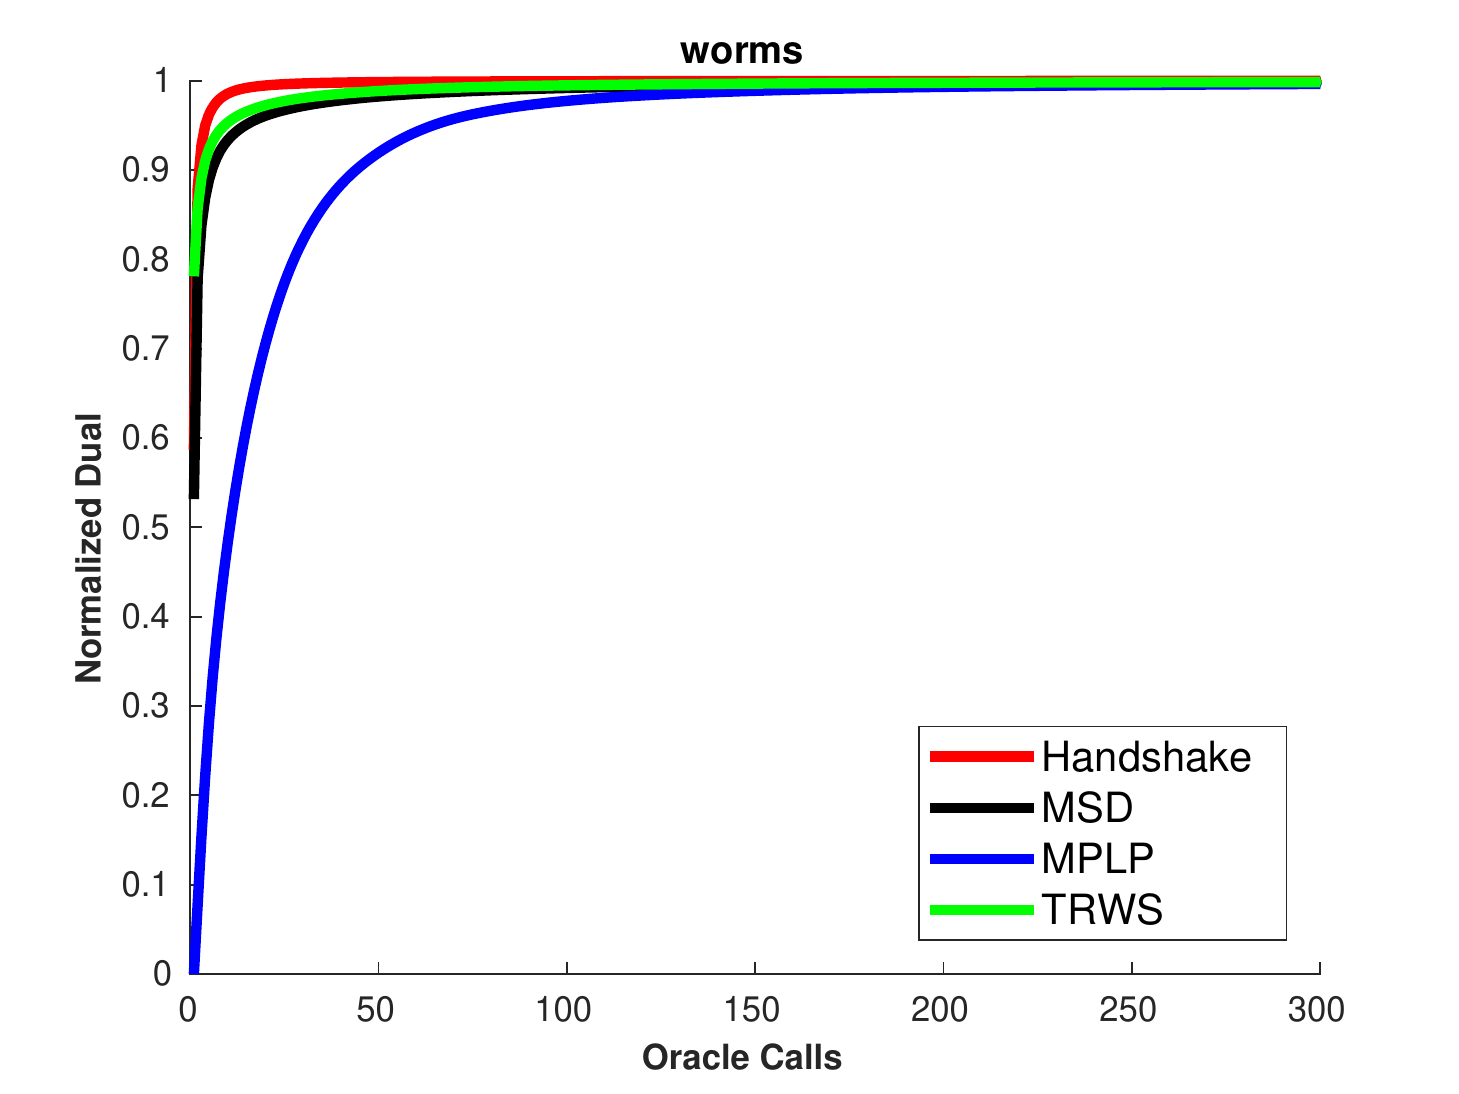}}
\end{subfigure}
\begin{subfigure}[Pose]{
\includegraphics[width=0.30\linewidth]{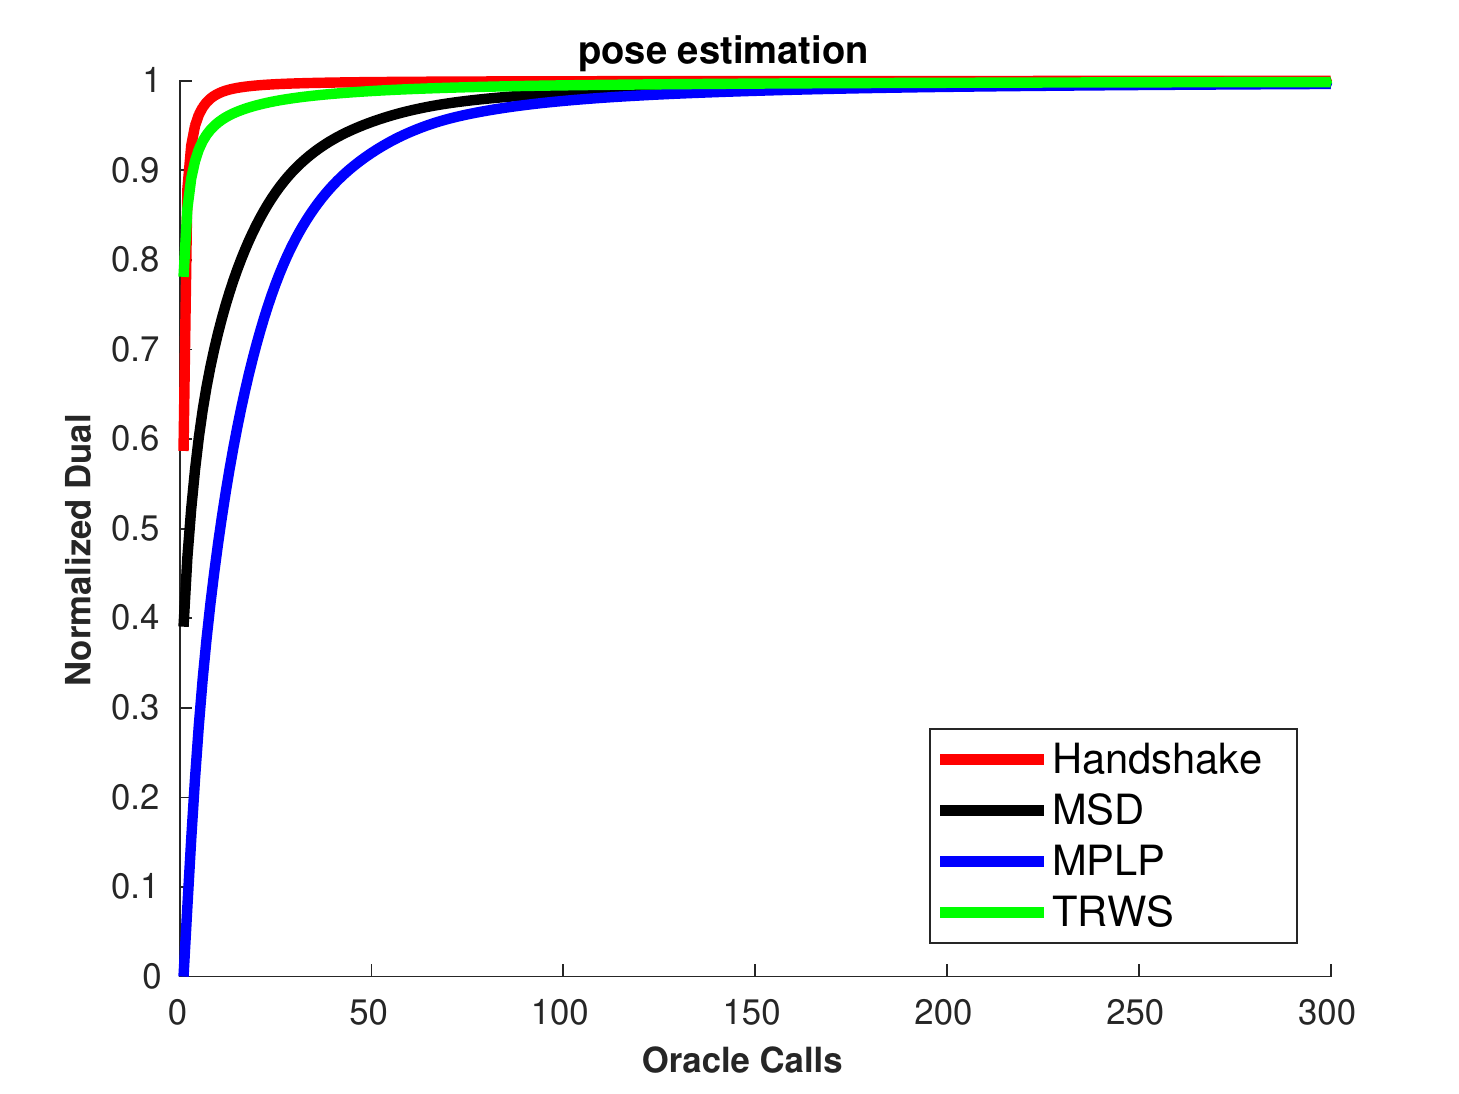}}
\end{subfigure}
%\begin{subfigure}[Stereo]{\includegraphics[width=0.18\linewidth]{plots/stereo/stereo_dual_iters}}
%\end{subfigure}
\begin{subfigure}[Color-Seg]{\includegraphics[width=0.30\linewidth]{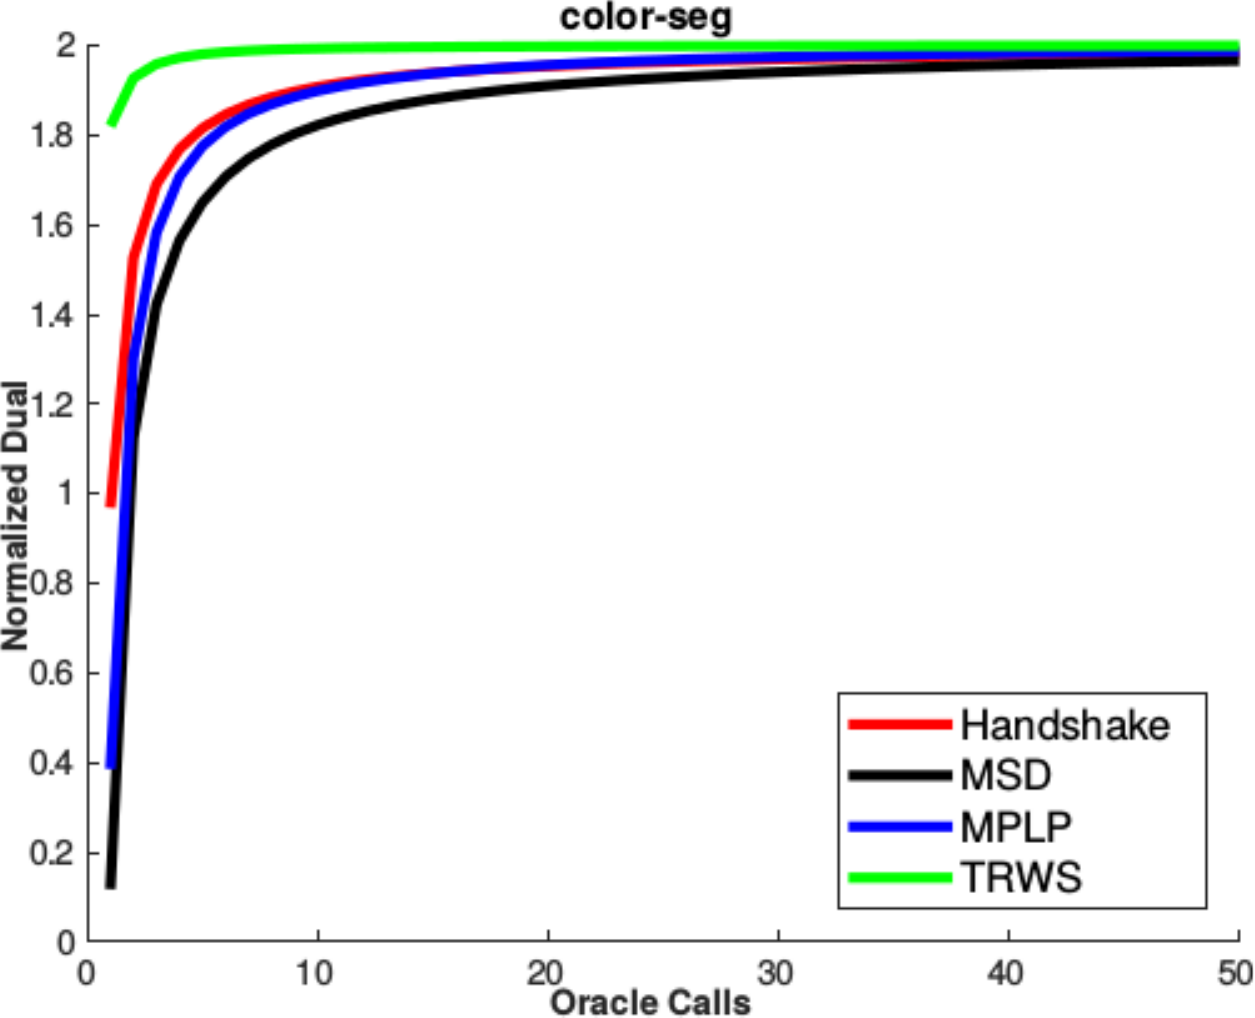}}
\end{subfigure}
\caption{Dual vs Oracle Calls: The algorithms we compare against have different message-passing schemes and end up doing different amounts of work per iteration. Thus instead of doing a straight forward plot of Dual versus iterations, we normalize the algorithms by the amount of work done per iteration. This is done by dividing each algorithm by it's oracle complexity, which measures the amount of work done per iteration in terms of messages passed. (a), (b) and (c) are dense graphs where \HaSh outperforms all other algorithms by a substantial margin. (d) and (e) on the other hand are on sparse graphs and \TRWS is dominant. Results are averaged over the entire dataset. The dual is normalized to 1 for equal weighing of every instance in the dataset.
}

\label{fig:dual_v_iters}
\end{figure*}

\begin{figure*}
\centering
%\begin{subfigure}[Protein Folding]
%{
%\includegraphics[width=0.18\linewidth]{plots/protein_folding/protein_folding_dual_time_st}
%}
%\end{subfigure}
\begin{subfigure}[Worms]{
\includegraphics[width=0.30\linewidth]{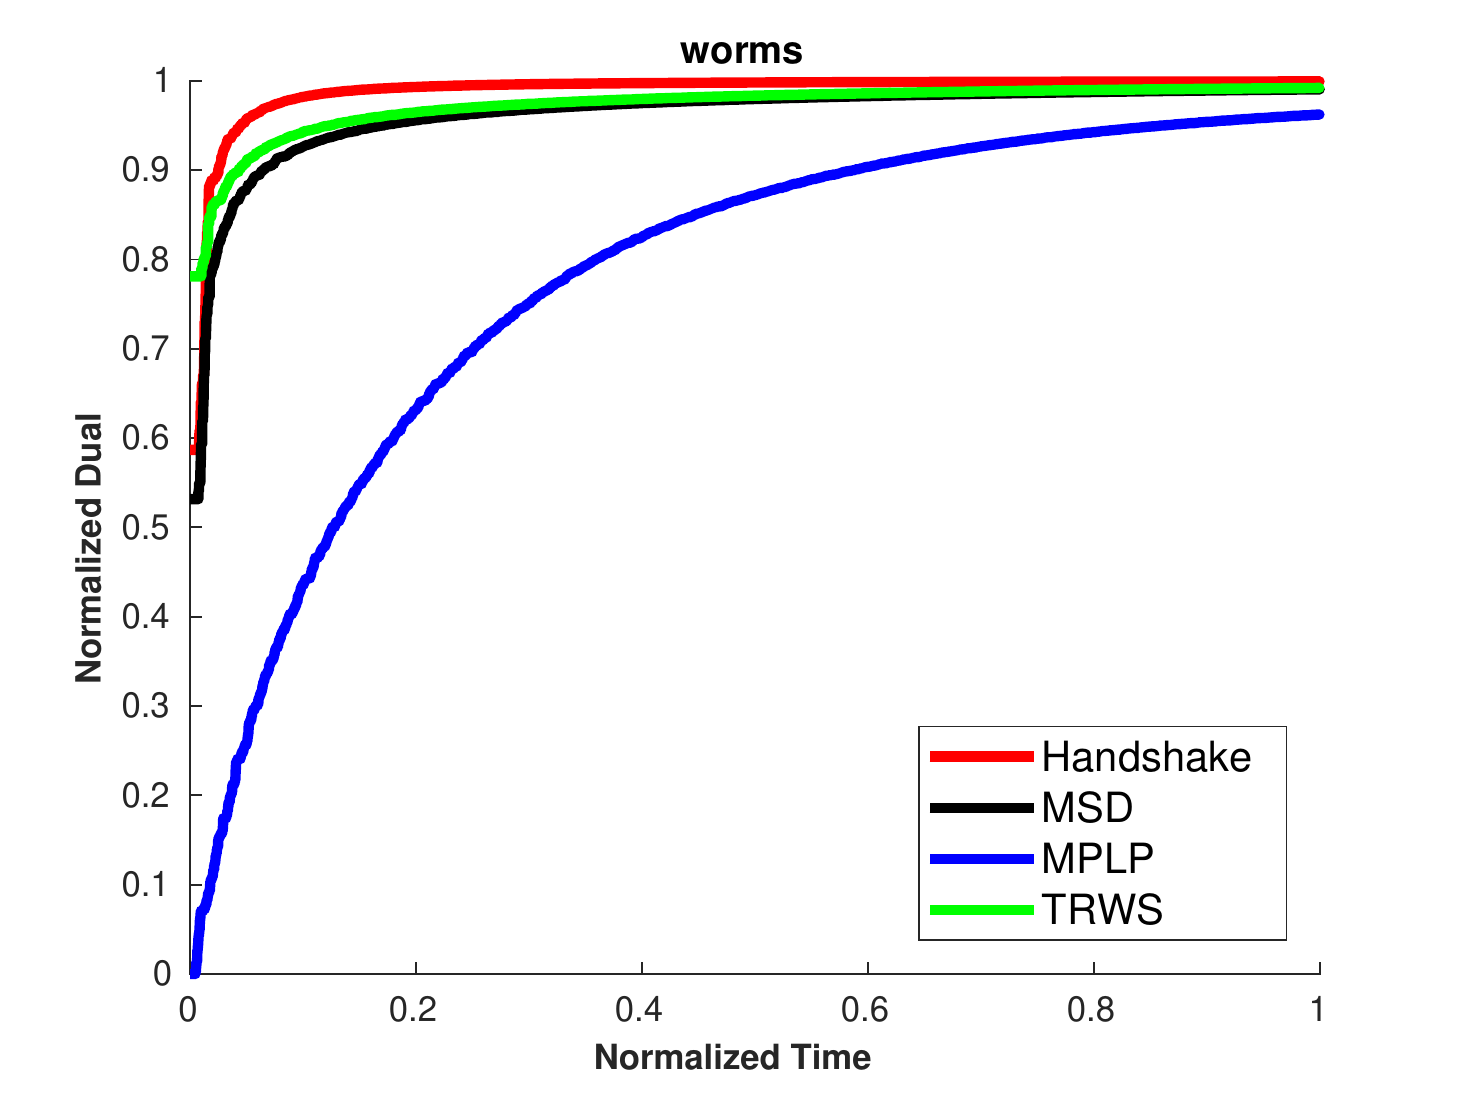}
}
\end{subfigure}
\begin{subfigure}[Pose]{
\includegraphics[width=0.30\linewidth]{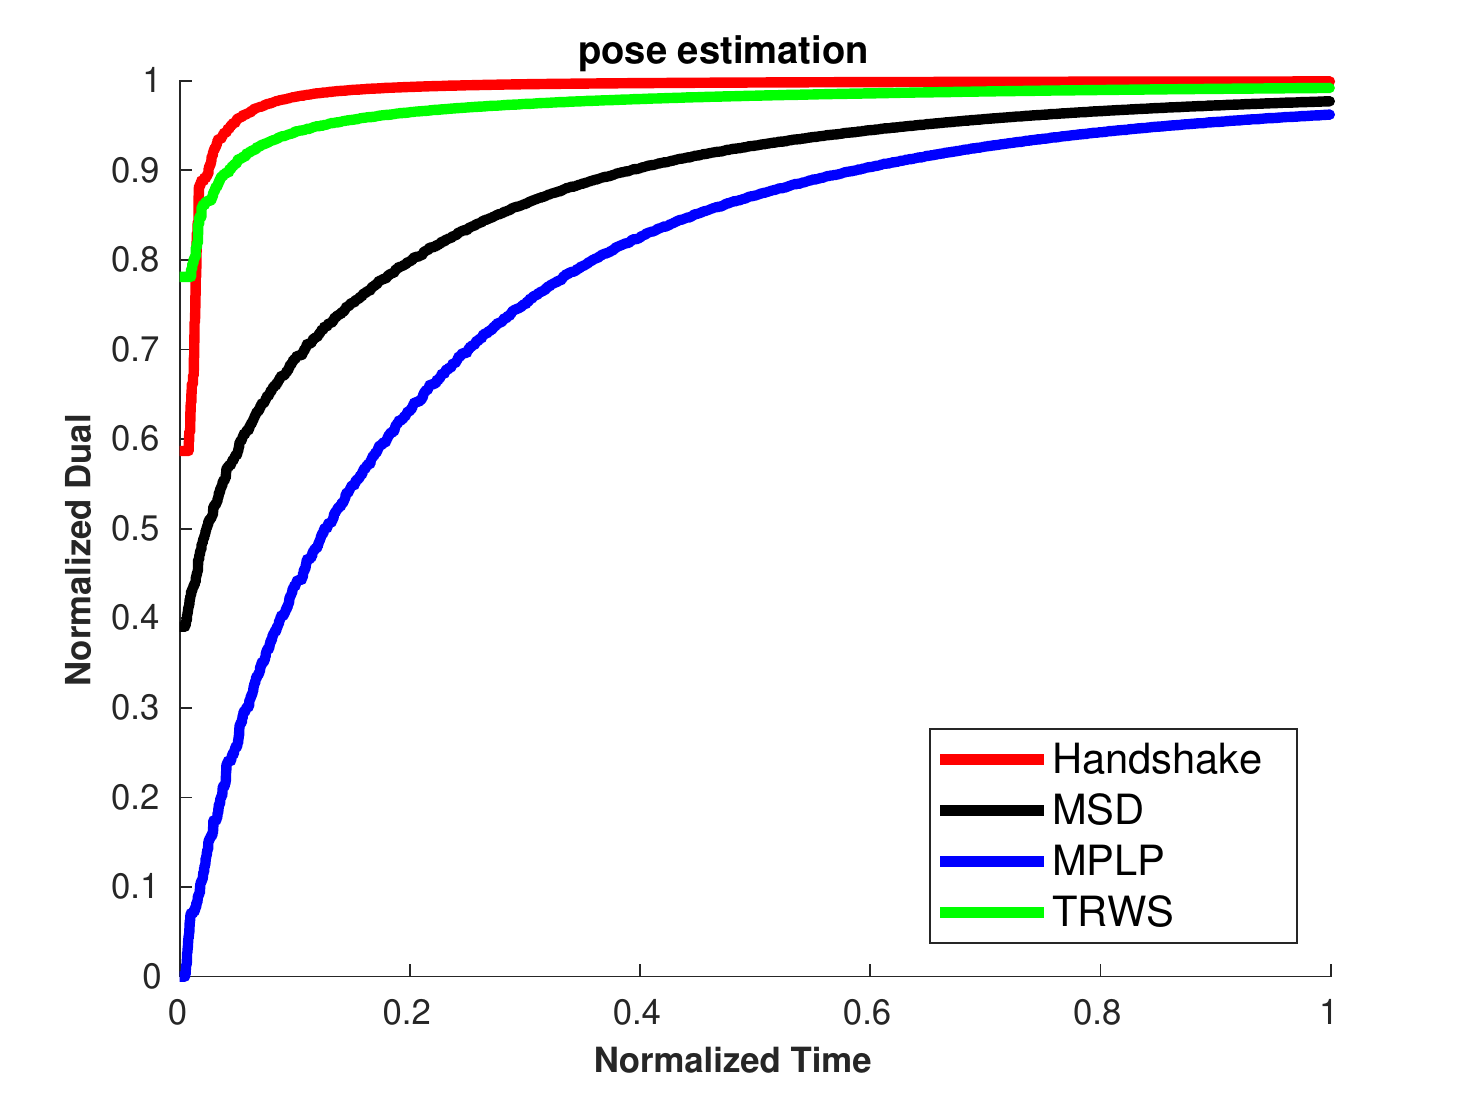}
}
\end{subfigure}
%\begin{subfigure}[Stereo]{
%\includegraphics[width=0.18\linewidth]{plots/stereo/stereo_dual_time_st}
%}
%\end{subfigure}
\begin{subfigure}[Color-Seg]{
\includegraphics[width=0.30\linewidth]{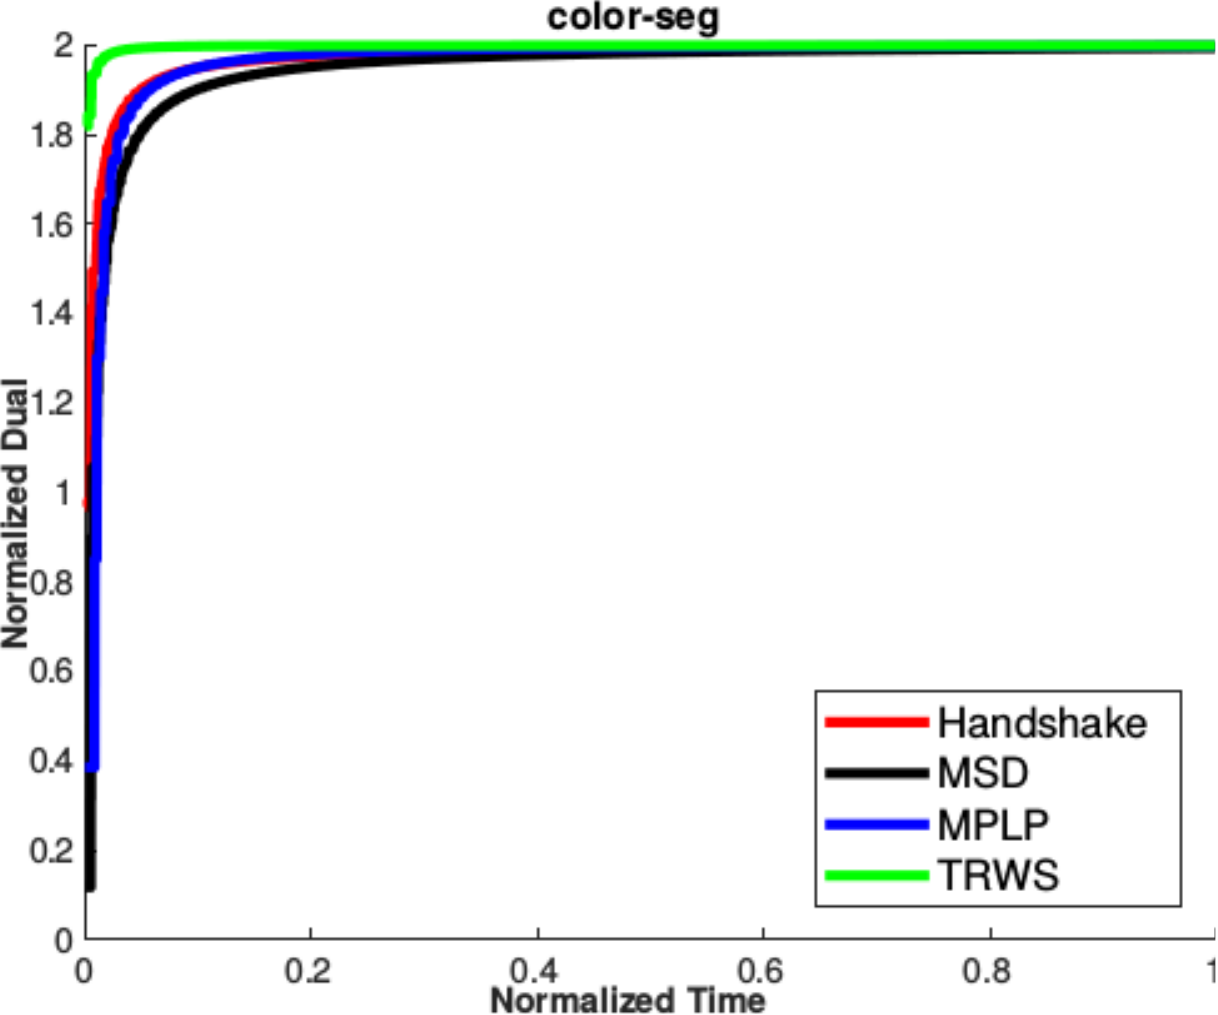}
}
\end{subfigure}

\caption{Dual vs Time (Single Threaded):  Fig. shows dual as a function of time for the single threaded versions of all the algorithms. Following the pattern in Fig. \ref{fig:dual_v_iters} for dense graphs (a), (b) and (c) \HaSh dominates all other algorithms by a considerable margin. For sparse graphs, (d) and (e) \TRWS is the fastest. Both the dual $D(\theta^\phi)$ and time have been averaged over the entire dataset and normalized to 1.The curves have been normalized such that each instance of the dataset is weighed equally.}
\label{fig:dual_v_time}
\end{figure*}

%\begin{figure*}
%\centering
%%\begin{subfigure}[Protein Folding]
%%{
%%\includegraphics[width=0.18\linewidth]{plots/protein_folding/protein_folding_dual_time_mt}
%%}
%%\end{subfigure}
%\begin{subfigure}[Worms]
%{
%\includegraphics[width=0.18\linewidth]{plots/worms/worms_dual_time_mt}
%}
%\end{subfigure}
%\begin{subfigure}[Pose]
%{
%\includegraphics[width=0.18\linewidth]{plots/pose_estimation/pose_estimation_dual_time_mt}
%}
%\end{subfigure}
%%\begin{subfigure}[Stereo]{
%%\includegraphics[width=0.18\linewidth]{plots/stereo/stereo_dual_time_mt}}
%%\end{subfigure}
%\begin{subfigure}[Color-Seg]{
%\includegraphics[width=0.18\linewidth]{plots/color_seg/color-seg_dual_time_mt}}
%\end{subfigure}
%\caption{Dual vs Time (Multi-Threaded): Figure shows dual $D(\phi)$ as a function of time for the algorithms with multi-threaded implementations, namely \HaSh and \TRWS. As in Fig. \ref{fig:dual_v_time} for dense graphs (a), (b) and (c) \HaSh dominates all other algorithms. The speedup due to parallelization is considerable compared to both the single threaded \MPLP and multi-threaded \TRWS. For sparse graphs (d) and (e) \TRWS beats all other algorithms. The normalization done for dual and time are the same as in Fig. \ref{fig:dual_v_time}.}
%\label{fig:dual_v_time_mt}
%\end{figure*}

%\input{experiments}
%\input{appendix}

%{\small
%\bibliographystyle{icml2017}
%\bibliography{handshake}
%}
%\section{Appendix}

\begin{figure*}
\centering
\begin{subfigure}[100$\%$]{\includegraphics[width=0.24\linewidth]{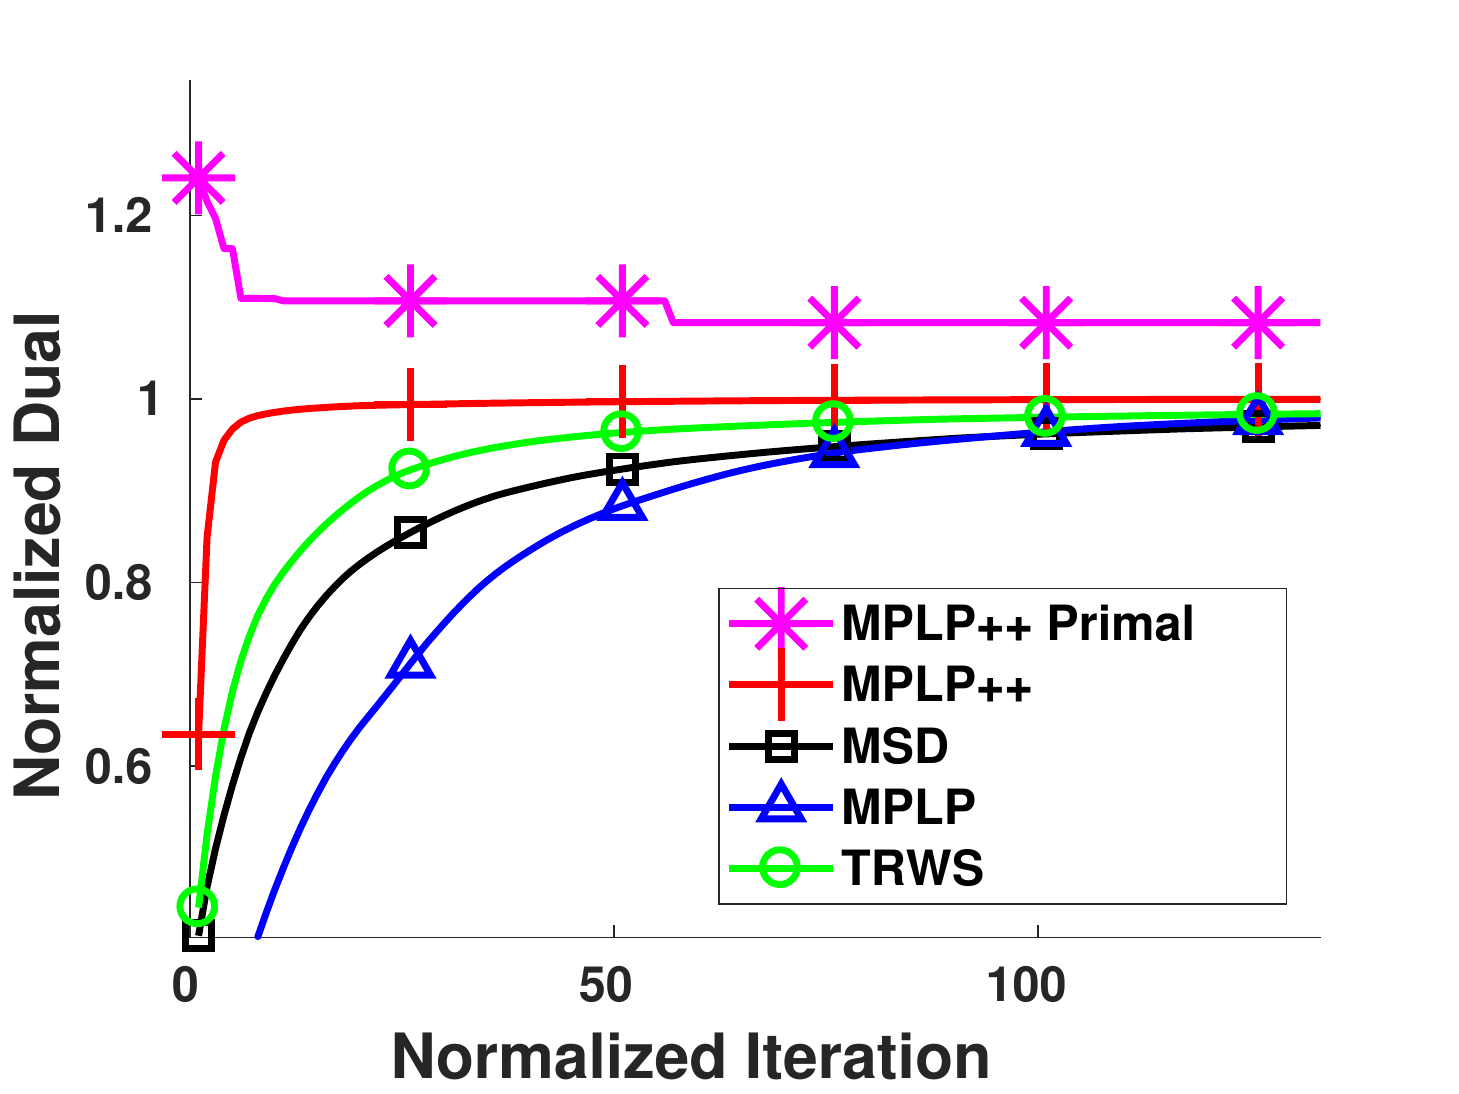}}
\end{subfigure}
\begin{subfigure}[80$\%$]{\includegraphics[width=0.24\linewidth]{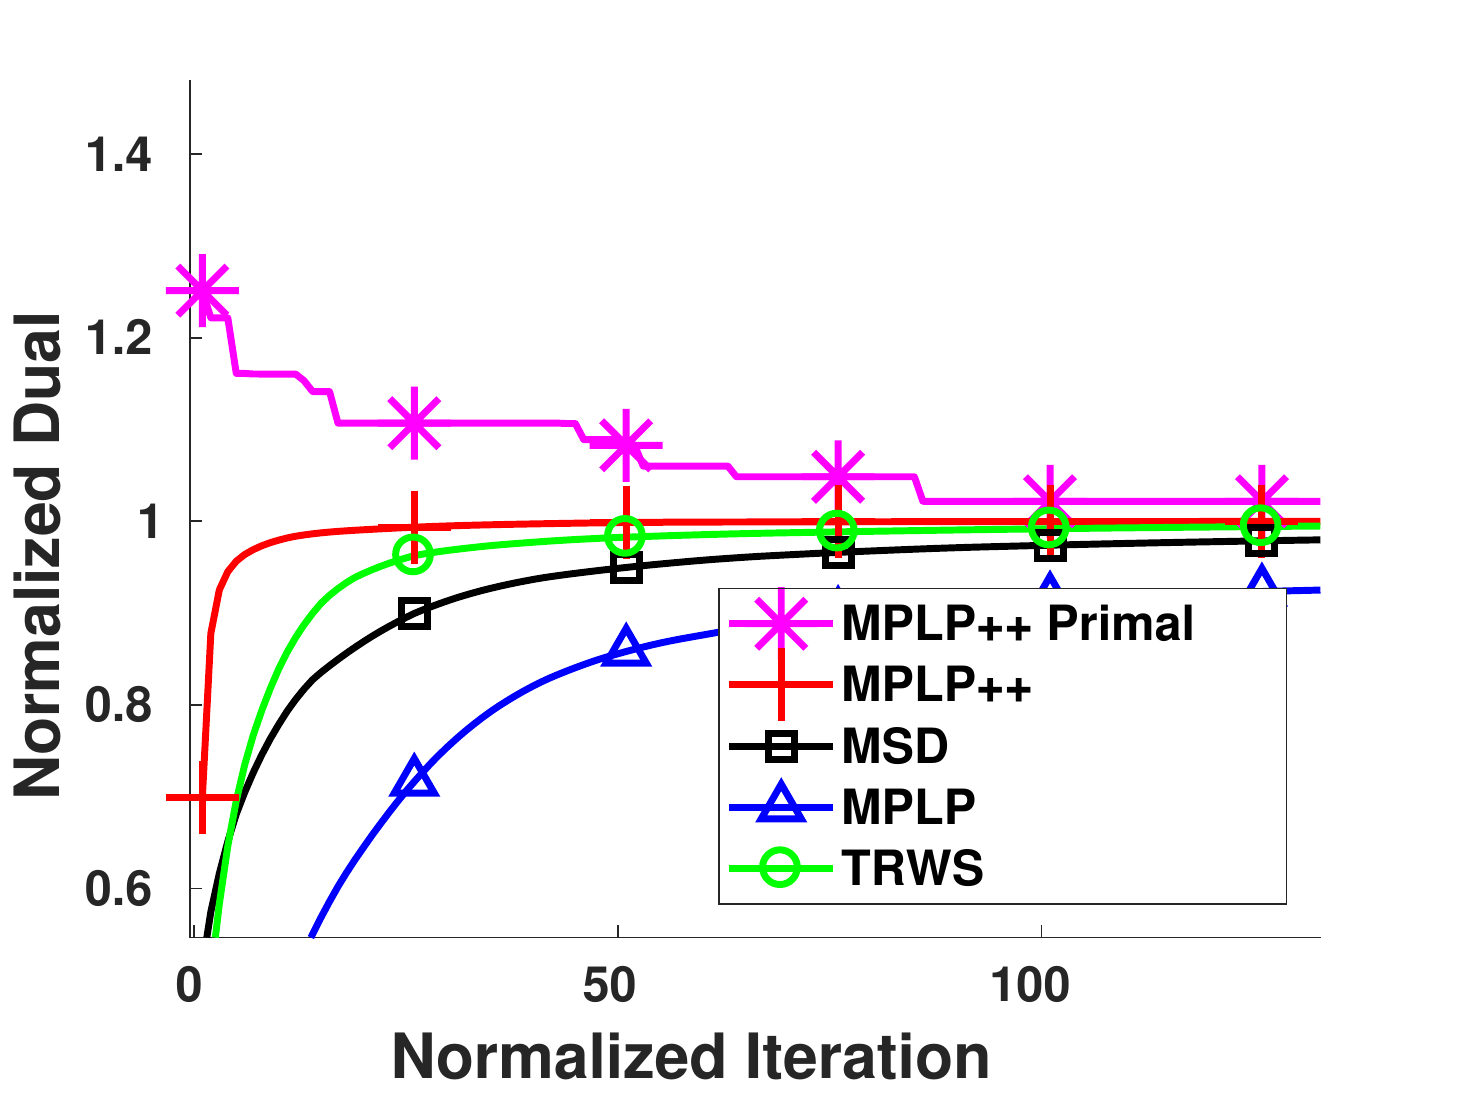}}
\end{subfigure}
\begin{subfigure}[60$\%$]{\includegraphics[width=0.24\linewidth]{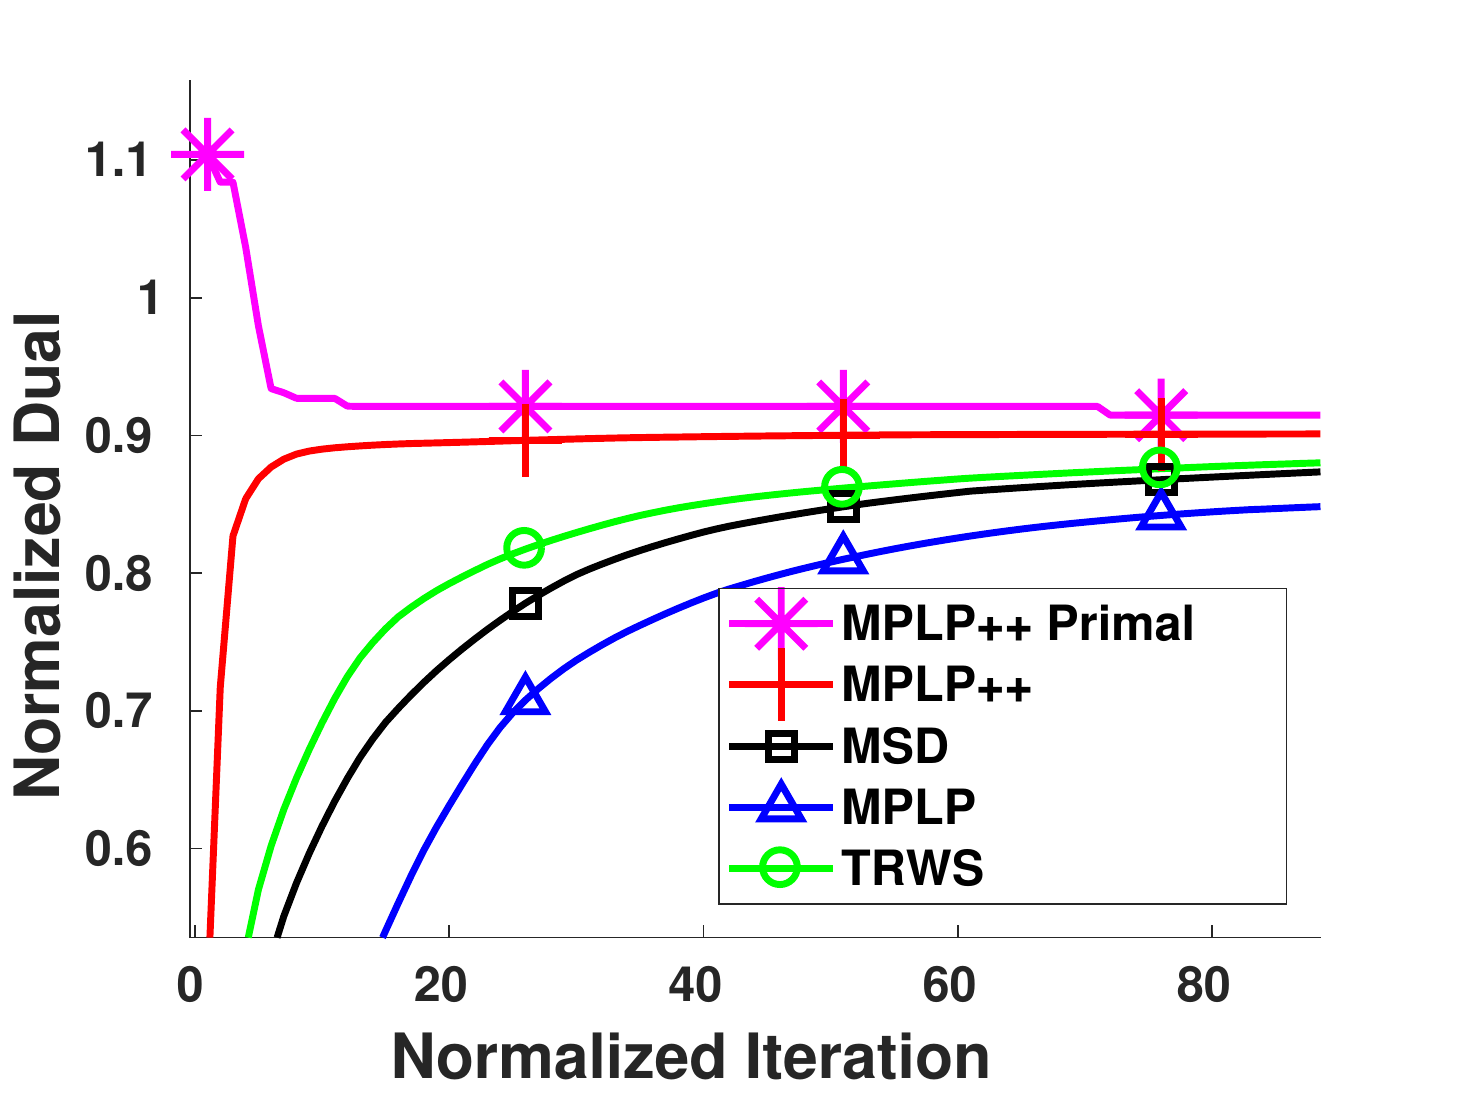}}
\end{subfigure}
\begin{subfigure}[40$\%$]{\includegraphics[width=0.24\linewidth]{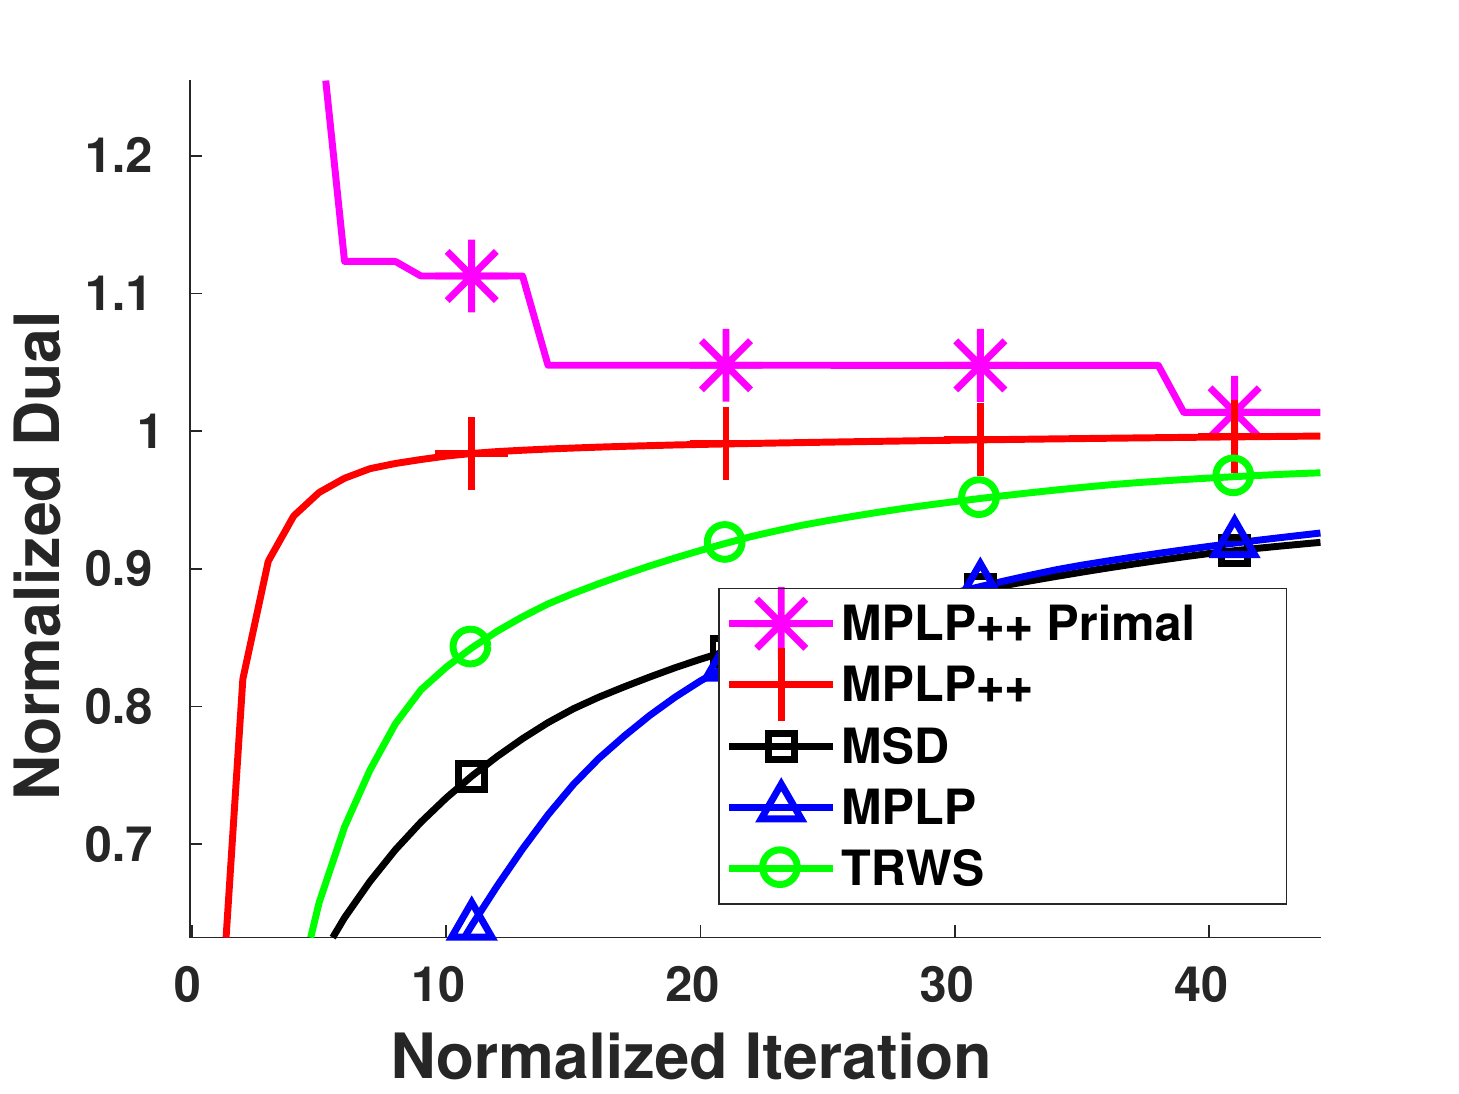}}
\end{subfigure}

\begin{subfigure}[20$\%$]
{\includegraphics[width=0.24\linewidth]{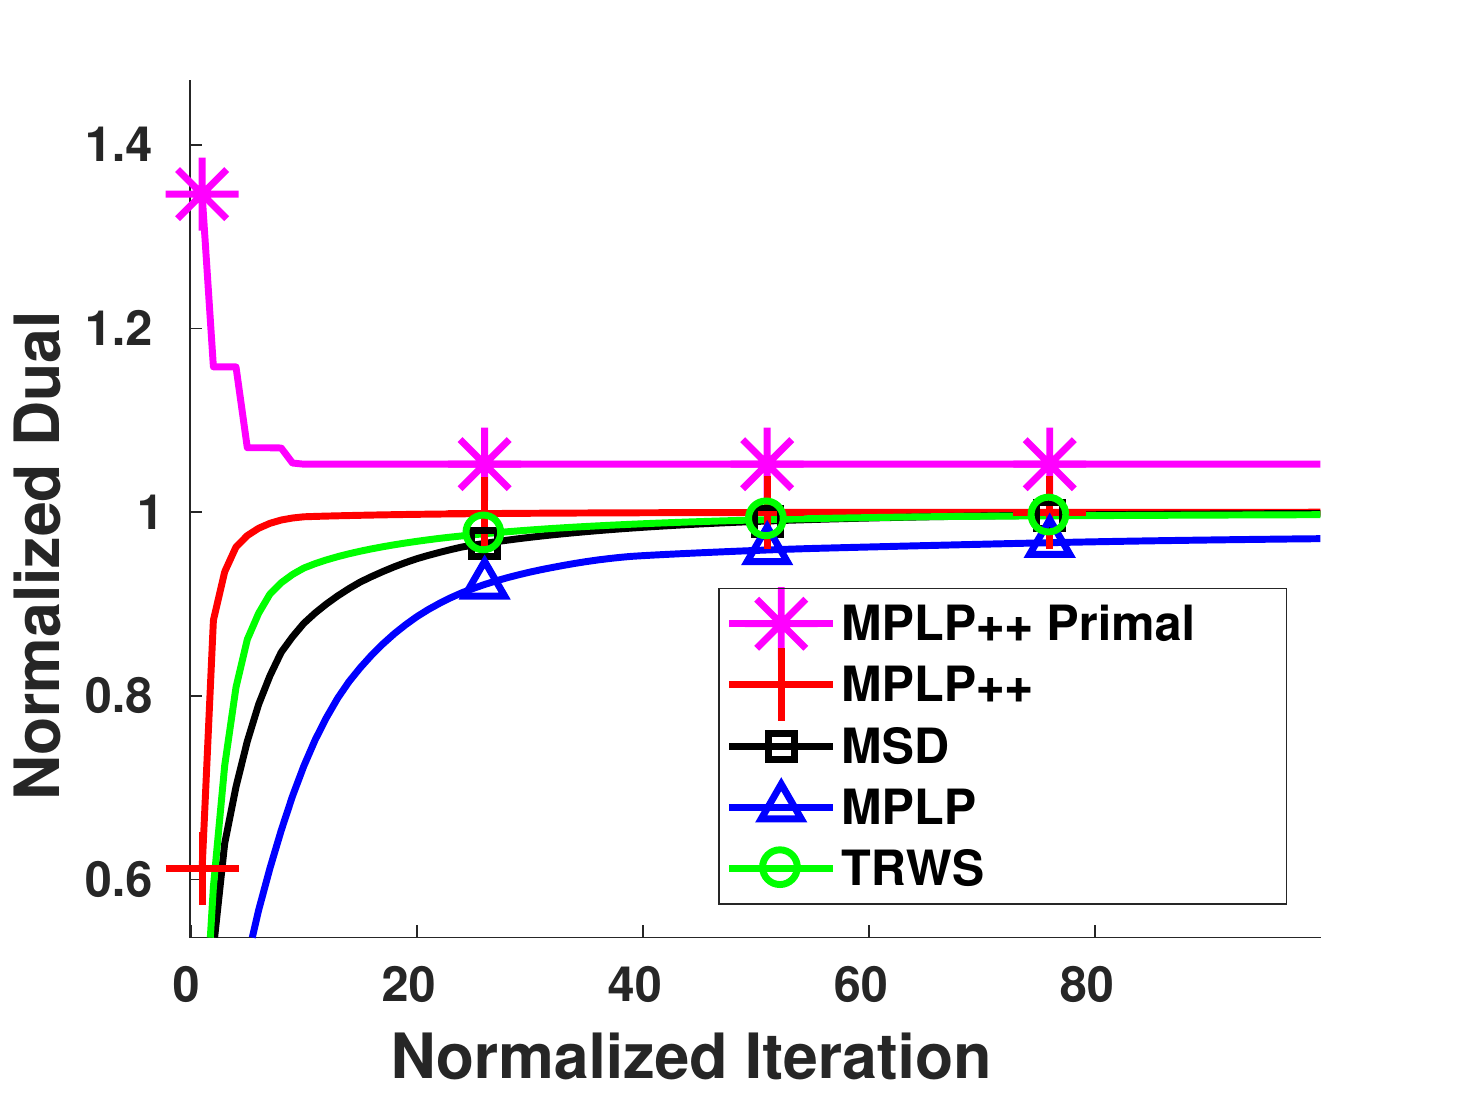}}
\end{subfigure}
\begin{subfigure}[10$\%$]
{\includegraphics[width=0.24\linewidth]{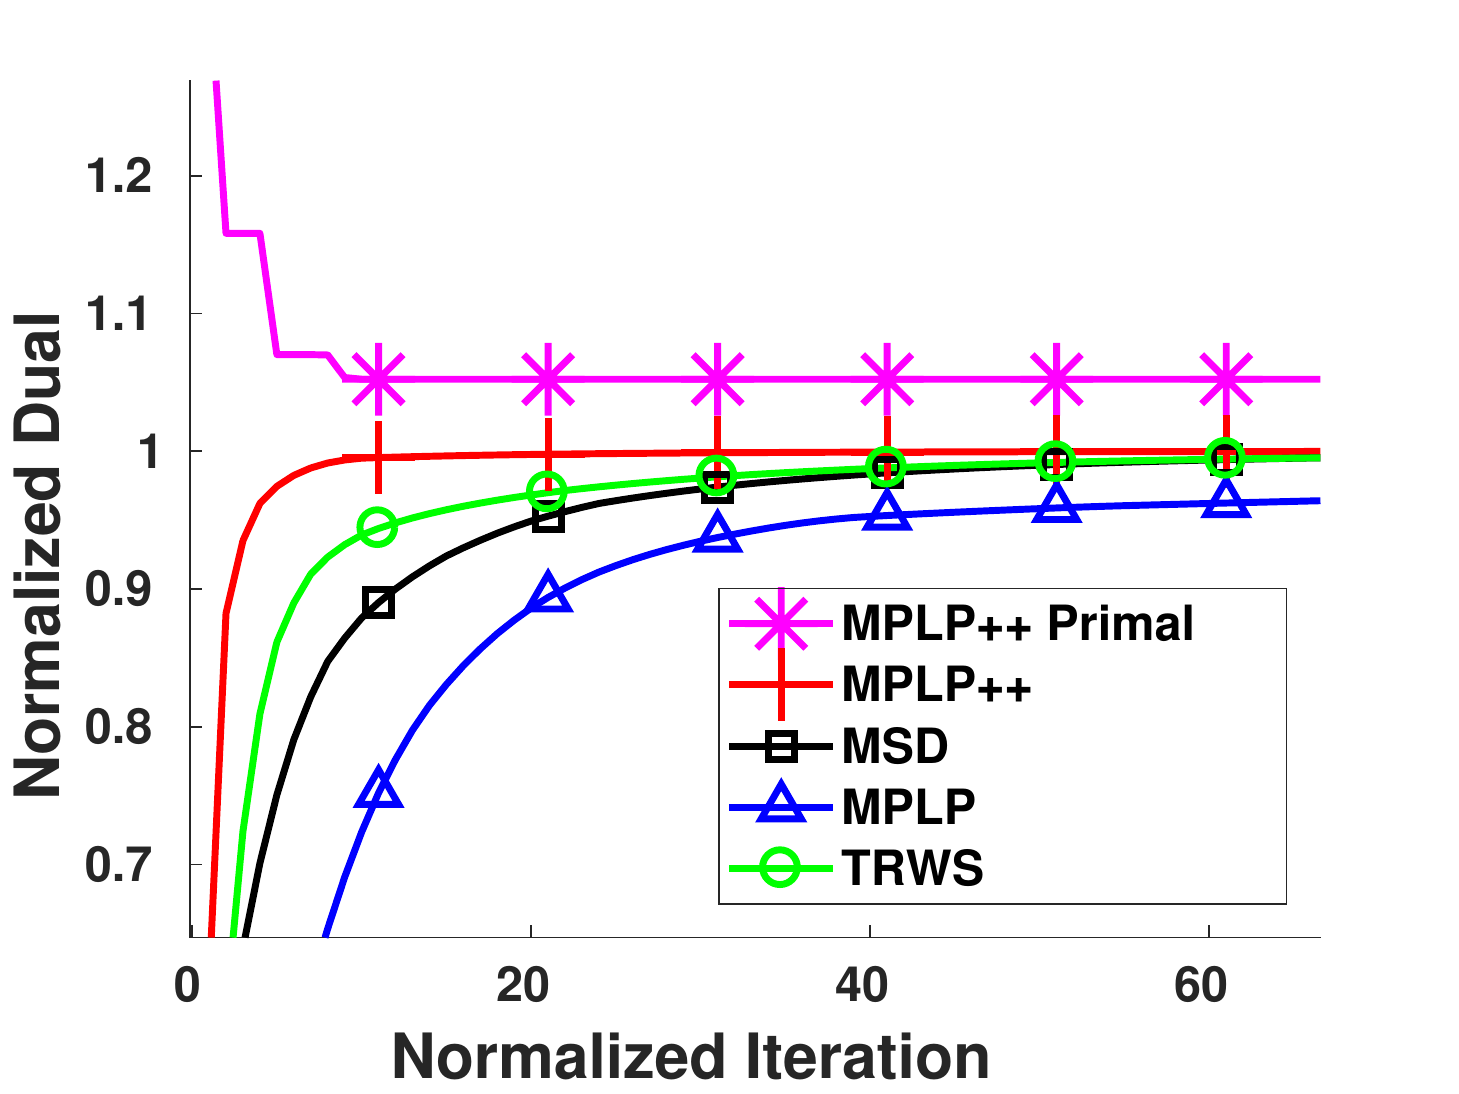}}
\end{subfigure}
\begin{subfigure}[5$\%$]
{\includegraphics[width=0.24\linewidth]{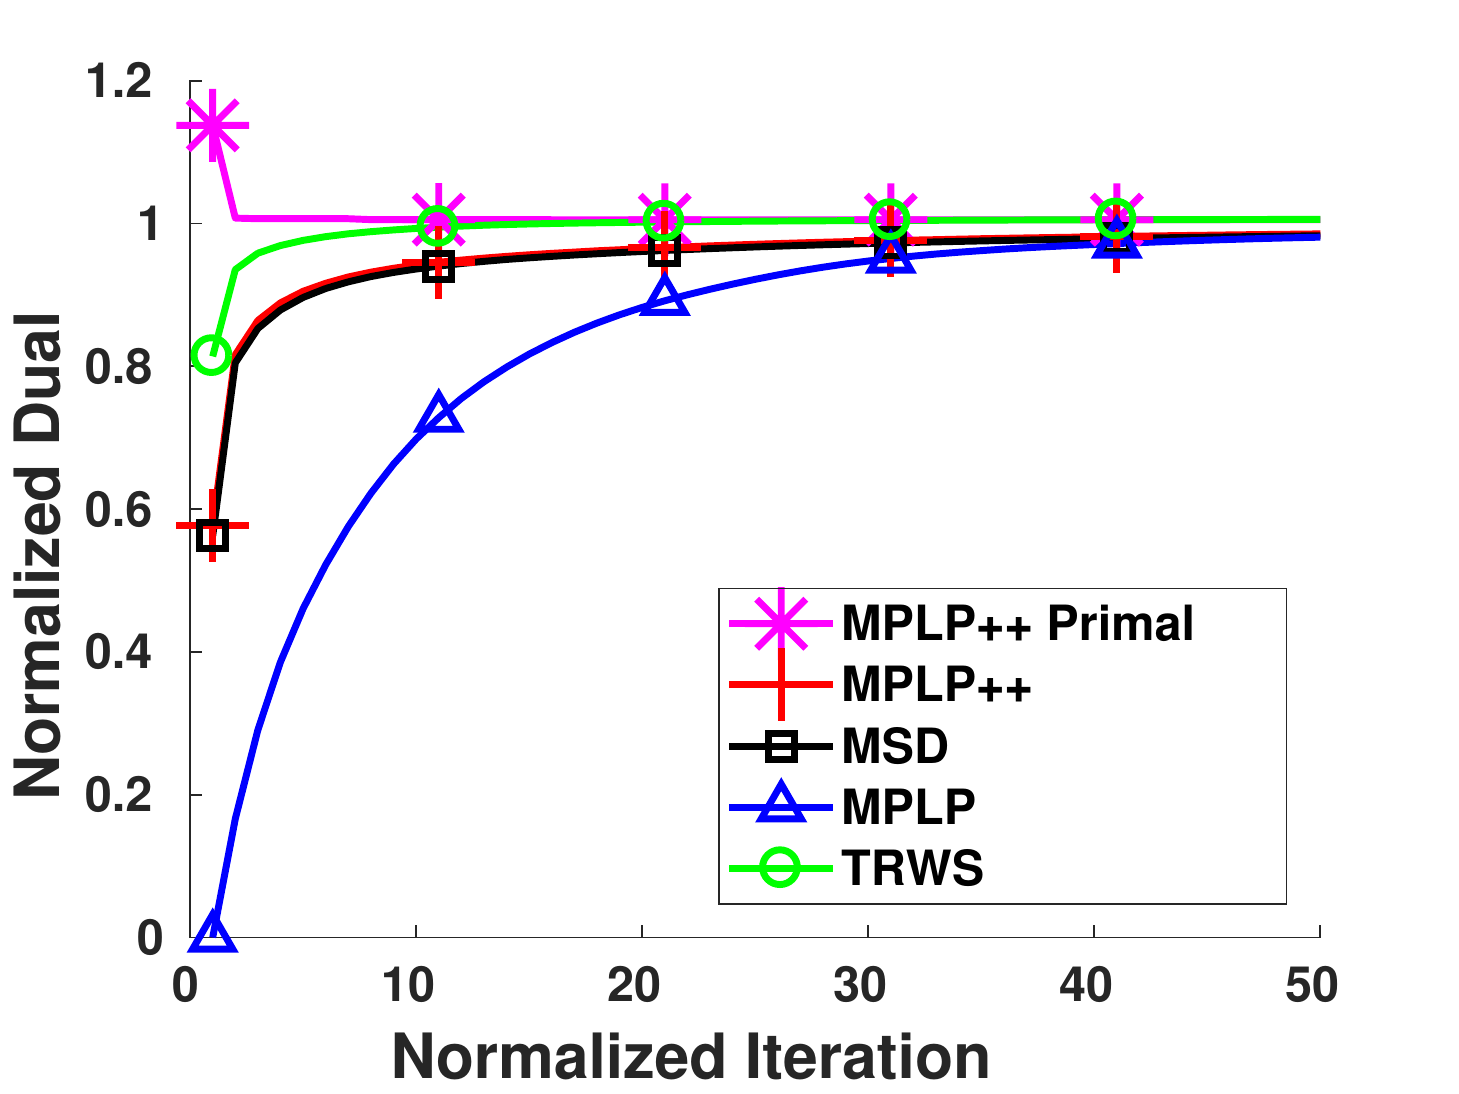}}
\end{subfigure}
\begin{subfigure}[1$\%$]
{\includegraphics[width=0.24\linewidth]{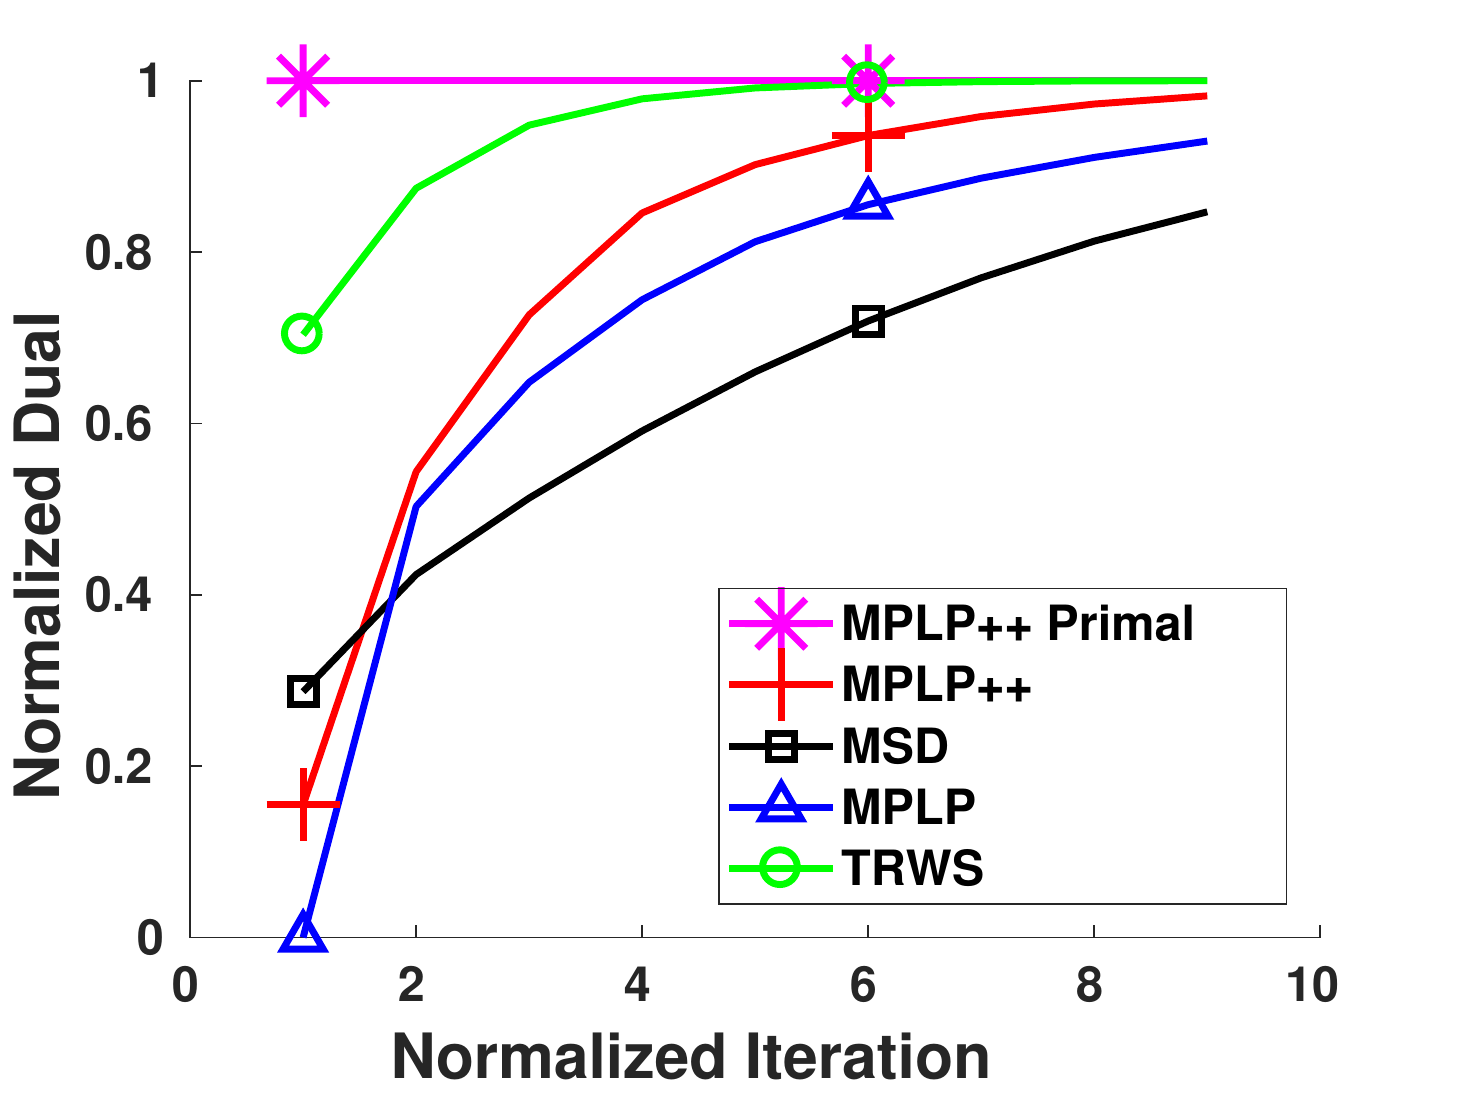}}
\end{subfigure}
\caption{\texttt{\textbf{Degradation With Sparsity (Dual vs Iterations): }}(a)-(h) show graphs with decreasing average connectivity given as percentage of possible edges in figure subcaption. In (a)-(f) \HaSh outperforms \TRWS. Handshake is resilient to graph sparsification even when 90$\%$ of the edges have been removed. For (g) and(h) \TRWS outperforms handshake.}
\label{fig:perf_deg_iter}
\end{figure*}

\begin{figure*}
\centering
\begin{subfigure}[Worms]{\includegraphics[width=0.32\linewidth]{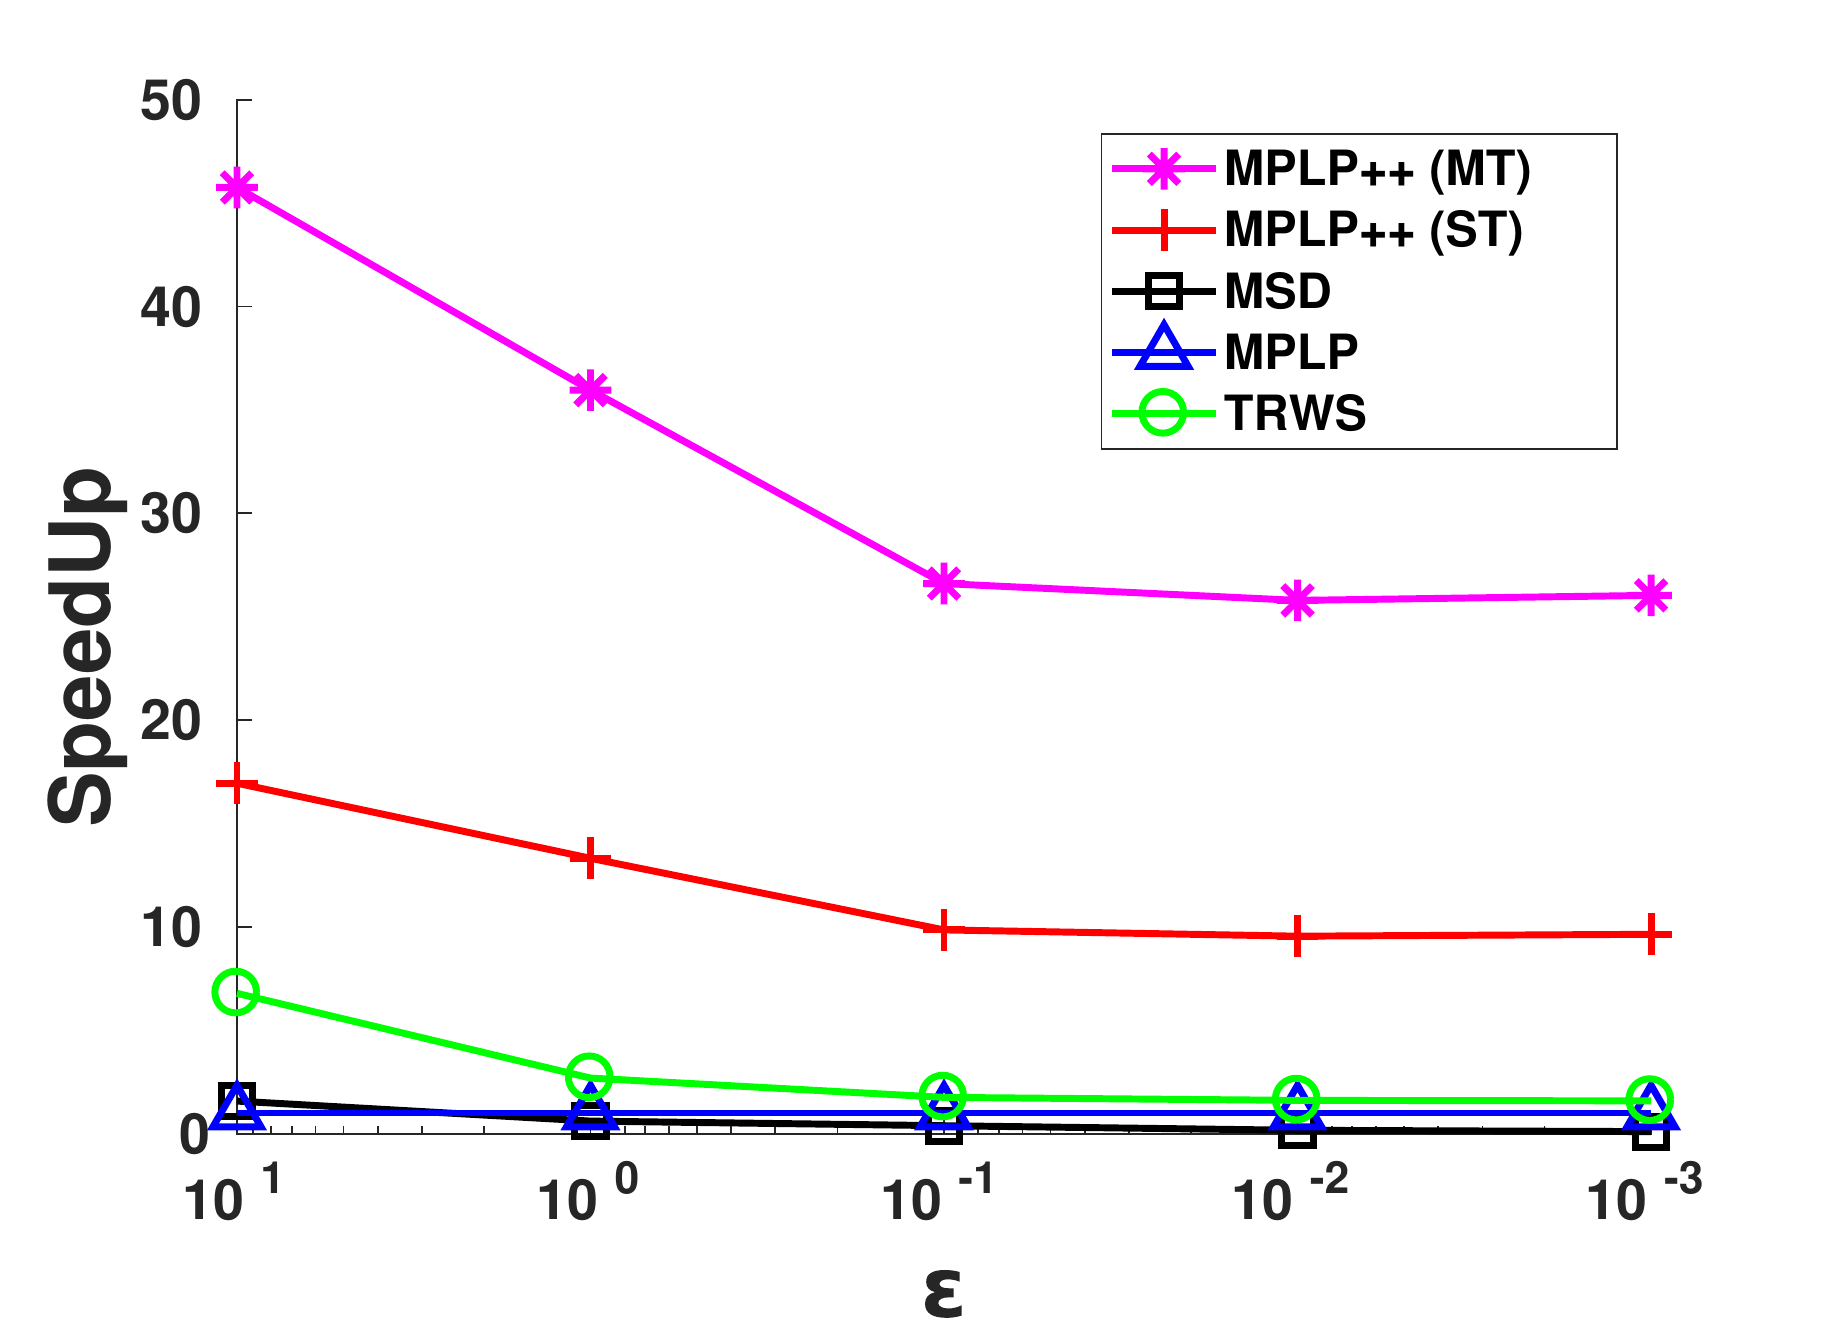}}
\end{subfigure}
\begin{subfigure}[Pose]
{\includegraphics[width=0.32\linewidth]{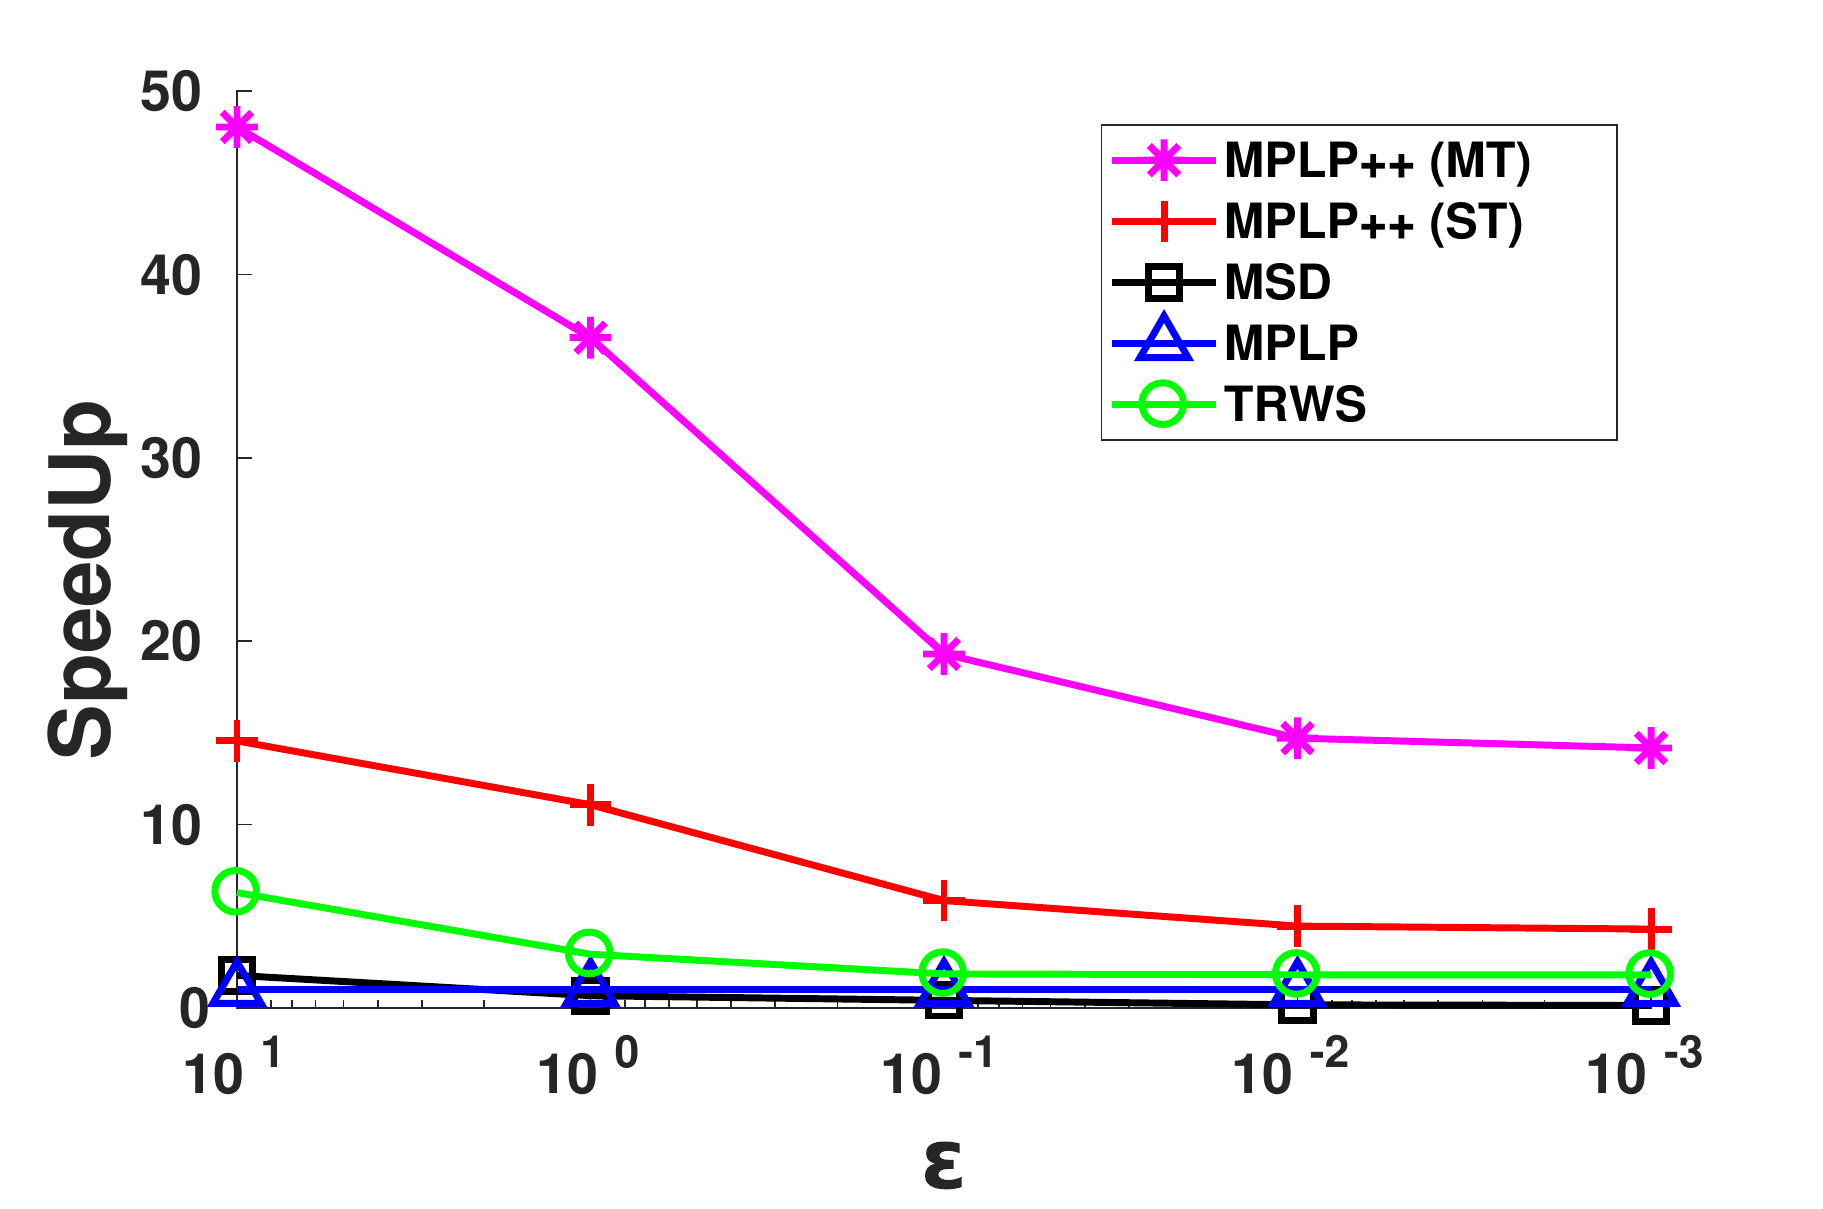}}
\end{subfigure}
\begin{subfigure}[Colorseg]
{\includegraphics[width=0.32\linewidth]{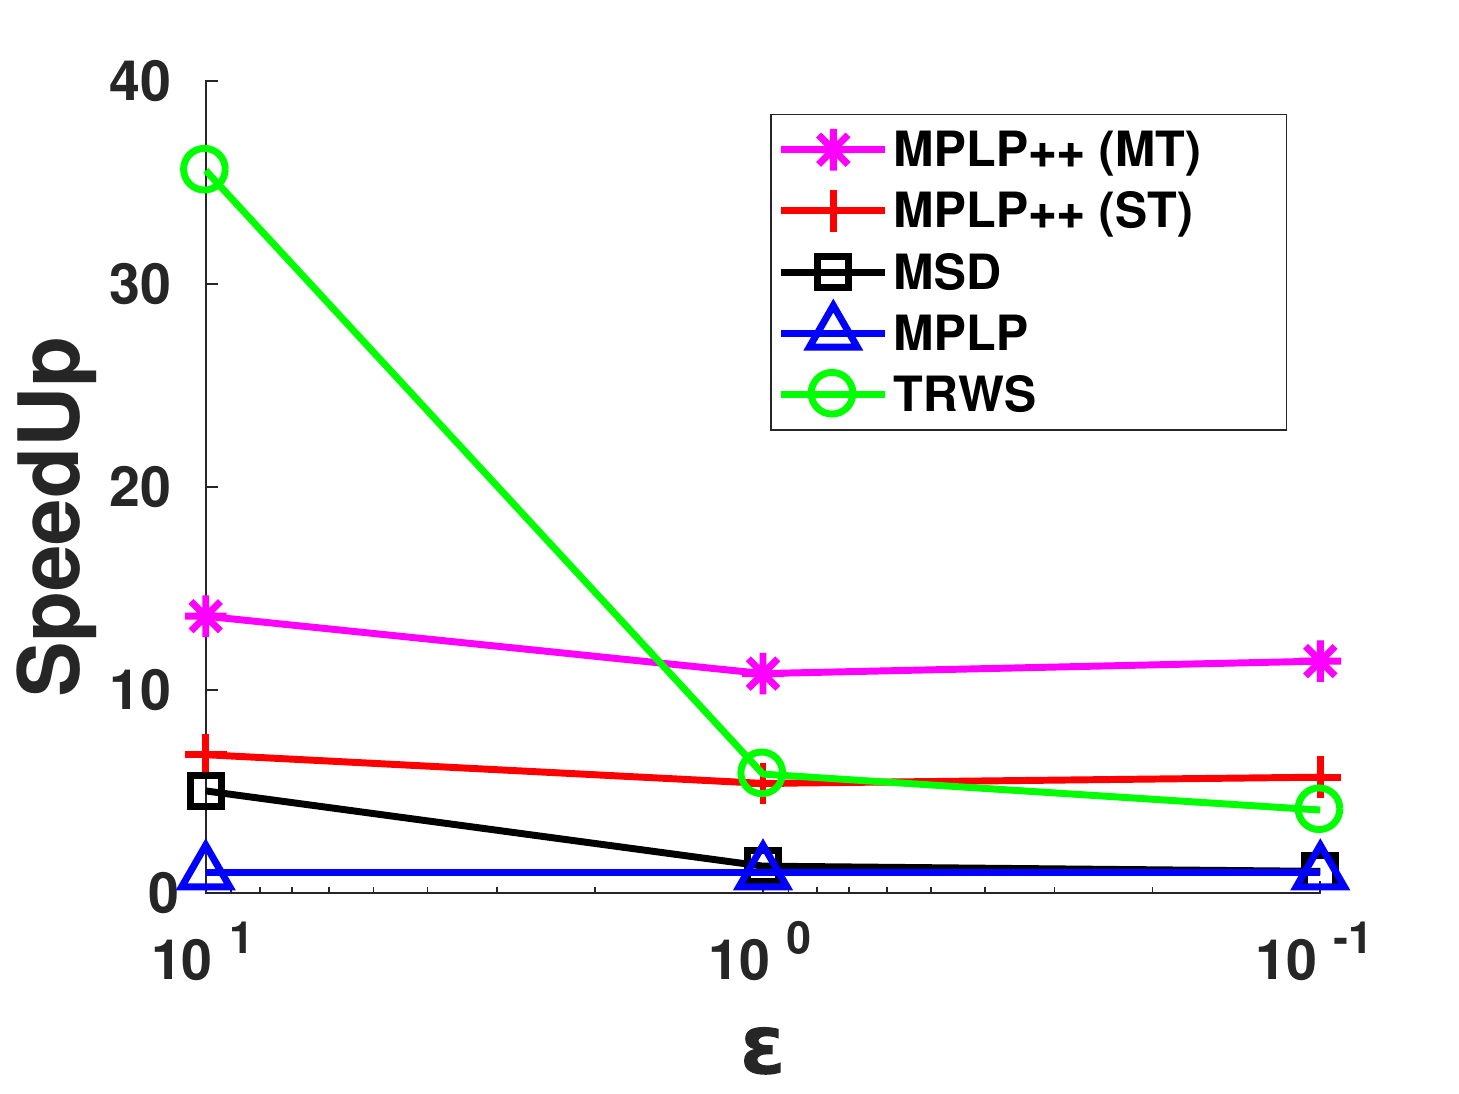}}
\end{subfigure}

\caption{Speedup comparisons with MPLP as the reference algorithm. The algorithms are run until
 Speedups are plotted for 3 $\epsilon$ 0.1,1.0}
\label{fig:speedups_dense}
\end{figure*}

\input{appendix}

%{\small
%\bibliographystyle{icml2017}
%\bibliography{handshake}
%}
%\section{Appendix}

\end{document}
